# Supplementary material for: Machine Translation Meta Evaluation through Translation Accuracy Challenge Sets
Source: arXiv:2401.16313 source file (2024-01-29)
Supplement: Supplementary file 1 [file zero_shot_appendix.tex]

\begin{table*}[t]
\small
\centering
\begin{tabular}{lcccccc}
\toprule
 &
  \multicolumn{2}{c}{\hyperref[sec:antonym]{\textbf{antonym-replacement}}} &
  \multicolumn{2}{c}{\begin{tabular}[c]{@{}l@{}}\hyperref[subsec:real-world-commonsense]{\textbf{real-world knowledge}}\\\hyperref[subsec:real-world-commonsense]{\textbf{-commonsense}}\end{tabular}} &
  \multicolumn{2}{c}{\hyperref[sec:nonsense]{\textbf{nonsense}}} \\
\midrule
 &
  \multicolumn{1}{c}{WMT} &
  \multicolumn{1}{c}{\begin{tabular}[c]{@{}l@{}}Non-\\  WMT\end{tabular}} &
  \multicolumn{1}{c}{WMT} &
  \multicolumn{1}{c}{\begin{tabular}[c]{@{}l@{}}Non-\\ WMT\end{tabular}} &
  \multicolumn{1}{c}{WMT} &
  \multicolumn{1}{c}{\begin{tabular}[c]{@{}l@{}}Non-\\ WMT\end{tabular}} \\
\midrule
BERTScore               & -0.376 & -0.408 & \phantom{-} 0.007 & \phantom{-} 0.060 & \phantom{-} 0.790  & -0.678 \\
BLEURT-20               & \phantom{-} 0.024  & -0.008 & \phantom{-} 0.396 & \phantom{-} 0.195 & -0.273 & -0.622 \\
COMET-20                & \phantom{-} 0.152  & \phantom{-} 0.104  & \phantom{-} 0.087 & \phantom{-} 0.020 & \phantom{-} 0.706  & -0.315 \\ 
COMET-QE                & \phantom{-} 0.616  & \phantom{-} 0.664  & \phantom{-} 0.168 & \phantom{-} 0.356 & \phantom{-} 0.245  & \phantom{-} 0.538  \\ \midrule
COMET-22                & \phantom{-} 0.744  & \phantom{-} 0.664  & \phantom{-} 0.584 & \phantom{-} 0.557 & \phantom{-} 0.706  & \phantom{-} 0.175  \\
metricx\_xl\_DA\_2019   & \phantom{-} 0.728  & \phantom{-} 0.760  & \phantom{-} 0.570 & \phantom{-} 0.624 & \phantom{-} 0.790  & \phantom{-} 0.357  \\
metricx\_xl\_MQM\_2020  & \phantom{-} 0.888  & \phantom{-} 0.936  & \phantom{-} 0.517 & \phantom{-} 0.611 & \phantom{-} 0.944  & \phantom{-} 0.762  \\
metricx\_xxl\_DA\_2019  & \phantom{-} 0.312  & \phantom{-} 0.296  & \phantom{-} 0.718 & \phantom{-} 0.758 & \phantom{-} 0.706  & \phantom{-} 0.441  \\
metricx\_xxl\_MQM\_2020 & \phantom{-} 0.696  & \phantom{-} 0.632  & \phantom{-} 0.691 & \phantom{-} 0.758 & \phantom{-} 0.930  & \phantom{-} 0.734  \\
UniTE-ref               & \phantom{-} 0.664  & \phantom{-} 0.696  & \phantom{-} 0.409 & \phantom{-} 0.396 & \phantom{-} 0.091  & -0.147 \\
UniTE                   & \phantom{-} 0.632  & \phantom{-} 0.552  & \phantom{-} 0.409 & \phantom{-} 0.409 & \phantom{-} 0.441  & -0.203 \\ \midrule
COMETKiwi               & \phantom{-} 0.744  & \phantom{-} 0.696  & \phantom{-} 0.745 & \phantom{-} 0.772 & \phantom{-} 0.510  & \phantom{-} 0.469  \\
Cross-QE                & \phantom{-} 0.680  & \phantom{-} 0.616  & \phantom{-} 0.638 & \phantom{-} 0.450 & \phantom{-} 0.720  & \phantom{-} 0.538  \\
HWTSC-Teacher-Sim       & \phantom{-} 0.504  & \phantom{-} 0.296  & \phantom{-} 0.248 & \phantom{-} 0.168 & \phantom{-} 0.930  & \phantom{-} 0.580  \\
UniTE-src               & \phantom{-} 0.776  & \phantom{-} 0.680  & \phantom{-} 0.651 & \phantom{-} 0.490 & \phantom{-} 0.524  & \phantom{-} 0.552  \\ 
 \bottomrule
\end{tabular}
\caption{Zero-shot performance of neural metrics on three phenomena to measure the ability of metrics to generalise to new language pairs. WMT language pairs consist of a subset of languages seen during training of the metrics, while non-WMT language pairs are unseen. Results show that the metrics are able to generalise to unseen languages. }
\label{tab:zero-shot-appendix}
\end{table*}
